# Supplementary material for: Coends of higher arity
Source: arXiv:2011.13881 source file (2020-11-27)
Supplement: Supplementary file 1 [file appendix.tex]

\section{Categorical Preliminaries}\label{appendix_catprel}
\ans{Is this appendix really necessary in the end? I mean: is \emph{everything} in it necessary? Also: we shall intersperse `$\clC$ is small' every now and then...}
\ansT{%
	Section by section:
	\begin{enumerate}
		\item Dinatural transformations: no; we moved this to examples (we need to finish the move tho);
		\item Parametric ends, diagonal functors, and Kan extensions: used in the co/kusarigamas section.
	\end{enumerate}
}
\subsection{Dinatural Transformations}
\begin{corollary}[The Yoneda lemma for dinatural transformations]\label{the-yoneda-lemma-for-dinatural-transformations}%
	Let $F,G\colon\clC^{\op}\times\clC\to \clD$ be functors.
	\begin{enumtag}{yd}
		\item\label{yd1}We have a natural bijection%
		%--- Begin Footnote ---%
		\footnote{%
			The authors learned this fact from a recent edit by \say{\href{https://nforum.ncatlab.org/account/1623/}{Hurkyl}} in \cite{nlab:dinatural-transformations}.
		}%
		%---  End Footnote  ---%
		\[\DiNat(F,G)\cong\Nat\left(\hom_{\clC}(-_{1},-_{2}),\hom_{\clC}\big(F^{-_{2}}_{-_{1}},G^{-_{1}}_{-_{2}}\big)\right).\]
		\item\label{yd2}%
		%--- Begin Footnote ---%
		\footnote{%
			This is is due to Street--Dubuc; see \cite[Theorem 1]{dinatural-transformations}.
		}%
		%---  End Footnote  ---%
		We have
		\begin{equation}\label{dinat-f-g-as-an-end}
			\DiNat(F,G)\cong\int_{A\in\clC}\hom_{\clD}\left(F^{A}_{A},G^{A}_{A}\right),
		\end{equation}
		where the \say{integrand} in \cref{dinat-f-g-as-an-end} is the functor%
		%--- Begin Footnote ---%
		\footnote{%
			It follows from \cref{p-q-ends-as-ordinary-ends} of \cref{prop:properties-of-p-q-ends} that we similarly have
			\begin{equation}\label{p-q-dinat-f-g-as-a-p-q-end}
				\pqDiNat{p}{q}(F,G)\cong\pqEnd{p}{q}{A\in\clC}\hom_{\clD}\left(F^{\bsA}_{\bsA},G^{\bsA}_{\bsA}\right),
			\end{equation}
			where the \say{integrand} in \cref{p-q-dinat-f-g-as-a-p-q-end} is now the functor
			\begin{diagram*}
				\begin{tikzcd}[row sep=0.0em, column sep=2.7em,  ampersand replacement=\&]
					\mathllap{\hom_{\clD}\left(F^{-_{2}}_{-_{1}},G^{-_{1}}_{-_{2}}\right)\colon}\pq{\clC}
					\arrow[r]
					\&
					\clD
					\\
					{(\bsA,\bsB)}
					\arrow[r, mapsto]
					\&
					{\hom_{\clD}\left(F^{\bsB}_{\bsA},G^{\bsA}_{\bsB}\right).}
				\end{tikzcd}
			\end{diagram*}%
		}%
		%---  End Footnote  ---%
		\begin{diagram*}
			\begin{tikzcd}[row sep=0.0em, column sep=2.7em,  ampersand replacement=\&]
				\mathllap{\hom_{\clD}\left(F^{-_{2}}_{-_{1}},G^{-_{1}}_{-_{2}}\right)\colon}\clC^{\op}\times\clC
				\arrow[r]
				\&
				\clD
				\\
				{(A,B)}
				\arrow[r, mapsto]
				\&
				{\hom_{\clD}\left(F^{B}_{A},G^{A}_{B}\right).}
			\end{tikzcd}
		\end{diagram*}%
		\item\label{ydp3}\cref{ydp1,ydp2} are equivalent.
	\end{enumtag}
\end{corollary}
\begin{proof}
	We divide the proofs by item:
	\begin{enumtag}{ydp}
		\item\label{ydp1}
		\item\label{ydp2}We have
		\item\label{ydp3}We have:
		\begin{enumtag}{yde}
			\item\cref{ydp1}$\implies$\cref{ydp2}: We have
			\item\cref{ydp2}$\implies$\cref{ydp1}: We have
			\begin{align*}
				\DiNat(F,G) & \cong \int_{A\in\clC}\hom_{\clD}\big(F^{A}_{A},G^{A}_{A}\big)                                                     \\
				            & \cong \int_{A,B\in\clC}\left[\hom_{\clC}(A,B),\hom_{\clD}\big(F^{B}_{A},G^{A}_{B}\big)\right]                     \\
				            & \cong \Nat\left(\hom_{\clC}(-_{1},-_{2}),\hom_{\clD}\big(F^{-_{2}}_{-_{1}},G^{-_{1}}_{-_{2}}\big)\right).\qedhere
			\end{align*}
		\end{enumtag}
	\end{enumtag}
\end{proof}
\subsection{Parametric ends}
Let $\clC$, $\clD$, and $\clE$ be categories, and let $F\colon\clC^{\op}\times\clC\times\clE\to \clD$ be a functor.
\begin{lemma}[{\cite[Theorems IX.7.2 and IX.7.3]{working-categories}}]\label{parametric-ends}\leavevmode%
	\begin{enumtag}{pe}
		\item\label{parametric-ends-1}Suppose that, for each $E\in\Obj(\clE)$, the end $\int_{A\in\clC}F^{A}_{A,E}$ of the functor $(A,A')\mapsto F^{A}_{A',E}$ exists. There exists a unique functor
		\[\textstyle\int F\colon\clE\to \clD\]
		such that, for each $E\in\Obj(\clE)$, we have
		\[\left(\textstyle\int F\right)_{E}=\int_{A\in\clC}F^{A}_{A,E}.\]
		\item\label{parametric-ends-2}$\int F$ is the end of the adjunct
		\[
			\begin{tikzcd}[row sep=0.0em, column sep=2.7em,  ampersand replacement=\&]
				\mathllap{\widehat{F}\colon}\clC^{\op}\times\clC
				\arrow[r]
				\&
				\left[\clE,\clD\right]
				\\
				(A,B)
				\arrow[r, mapsto]
				\&
				F^{A}_{B,-_{1}}
			\end{tikzcd}
		\]
		of $F$ under the adjunction $(-)\times(-)\dashv\left[\clE,\clD\right]$ of $\Cats$.
	\end{enumtag}
\end{lemma}
\begin{definition}\label{def:parametric-end}
	The \emph{parametric end} of $F$ is, if it exists, the functor $\int F$ of \cref{parametric-ends}.
\end{definition}
% \subsection{Dummy functors}
% \begin{notation}\label{not:dummy}
% 	We say that
% 	\begin{itemize}
% 		\item A functor $F : \pq{\clC}[p+r][q+s] \to \clD$ is $(r,s)$-\emph{dummy} if it factors through the canonical projection $\pi_{r,s} : \pq{\clC}[p+r][q+s] \to \pq{\clC}$ that cancels the last $r$ contravariant components, and the last $s$ covariant components.
% 		\item Given a functor $F : \pq{\clC} \to \clD$ we define its $(r,s)$-\emph{dummyfication} to be the composition $\overline{F} : \pq{\clC}[p+r][q+s] \xrightarrow{\pi_{r,s}} \pq{\clC} \xrightarrow{F} \clD$; this promotes every functor of type $\left[\pqMat{p\\q}\right]$ to an $(r,s)$-dummy one.
% 	\end{itemize}
% 	It's obvious that every functor that is mute in \emph{some} of its variables can be made into an $(r,s)$-dummy one by suitably reshuffling its arguments.
% \end{notation}
\subsection{Diagonal Functors}
Let $\clC$ be a category.
\begin{definition}
	The \emph{diagonal functor} of $\clC$ is the functor
	\begin{diagram*}
		\begin{tikzcd}[row sep=0.0em, column sep=2.7em,  ampersand replacement=\&]
			\mathllap{\Delta\colon}\clC
			\arrow[r]
			\&
			\clC\times\clC
			\\
			A
			\arrow[r, mapsto]
			\&
			(A,A)\mrp{.}
			\\
		\end{tikzcd}
	\end{diagram*}%
\end{definition}
\begin{proposition}[Adjoints to the Diagonal Functor]
	If $\clC$ has products and coproducts, then we have a triple adjunction
	\begin{center}
		$\left(\coprod\dashv\Delta\dashv\times\right)\colon\phantom{\clC\times}$
		\begin{tikzcd}[row sep=4.5em, column sep=4.5em, background color=backgroundColor]
			\mathllap{\clC{}\times{}}\clC
			\arrow[r, "\coprod"{name=Lan}, shift left=1.5em]
			\arrow[r, "\times"'{name=Ran}, shift right=1.5em]
			&
			\clC\mathrlap{.}
			\arrow[l, "\Delta"{name=K,description}]
			%--- adjunction symbols
			\arrow[phantom,from=K, to=Lan,"\dashv" rotate=-90]
			\arrow[phantom,from=K, to=Ran,"\dashv" rotate=-90]
		\end{tikzcd}
	\end{center}%
\end{proposition}
\begin{proof}%
	The proposition follows from the universal property of the co/product, as we have bijections
	\[\hom_{\clC}\left(A\textstyle\coprod B,C\right)\cong\hom_{\clC\times\clC}\left((A,B),(C,C)\right)\cong\hom_{\clC}\left(A,B\times C\right),\]
	natural in $A,B,C\in\clC_o$.
\end{proof}
